# Supplementary material for: Estimating the lifetime risk of a false positive screening test result
Source: arXiv:2206.08463 ancillary file (2022-06-16)
Supplement: Supplementary file 1 [file supplementary_material.pdf]

# Estimating the lifetime risk of a false positive screening test result

## Supplementary material

Tim White and Sara Algeri

## Table S1: Inclusion criteria for each disease

| Disease | Date of most recent USPSTF screening recommendation as of August 31, 2021 | Cancer, STD, or neither | USPSTF grade of C or higher for at least some individuals | Included in analysis |
|---|---|---|---|---|
| Breast cancer | February 2016[1] | Cancer[2] | Yes[1] | Yes |
| Cervical cancer | August 2018[3] | Cancer[2] | Yes[3] | Yes |
| Chlamydia | December 2014[4] | STD[5] | Yes[4] | Yes |
| Colorectal cancer | May 2021[6] | Cancer[2] | Yes[6] | Yes |
| Gonorrhea | December 2014[4] | STD[5] | Yes[4] | Yes |
| Hepatitis B | December 2020[7] and July 2019[8] | STD[5] | Yes[7,8] | Yes |
| Hepatitis C | March 2020[9] | STD[5] | Yes[9] | Yes |
| HIV | June 2019[10] | STD[5] | Yes[10] | Yes |
| Lung cancer | March 2021[11] | Cancer[2] | Yes[11] | Yes |
| Prostate cancer | May 2018[12] | Cancer[2] | Yes[12] | Yes |
| Syphilis | June 2016[13] and September 2018[14] | STD[5] | Yes[13,14] | Yes |
| Abdominal aortic aneurysm | December 2019[15] | Neither[2,5] | Yes[15] | No |
| Asymptomatic bacteriuria | September 2019[16] | Neither[2,5] | Yes[16] | No |
| Bladder cancer | August 2011[17] | Cancer[2] | No[17] | No |
| Depression | March 2016[18] and January 2016[19] | Neither[2,5] | Yes[18,19] | No |
| Genital herpes | December 2016[20] | STD[5] | No[20] | No |
| Gestational diabetes | August 2021[21] | Neither[2,5] | Yes[21] | No |
| Hypertension | April 2021[22] | Neither[2,5] | Yes[22] | No |

| | | | | |
|---|---|---|---|---|
| Intimate partner violence, elder abuse, and abuse of vulnerable adults | October 2018[23] | Neither[2,5] | Yes[23] | No |
| Latent tuberculosis | September 2016[24] | Neither[2,5] | Yes[24] | No |
| Oral cancer | January 2014[25] | Cancer[2] | No[25] | No |
| Osteoporosis | June 2018[26] | Neither[2,5] | Yes[26] | No |
| Ovarian cancer | February 2018[27] | Cancer[2] | No[27] | No |
| Pancreatic cancer | August 2019[28] | Cancer[2] | No[28] | No |
| Prediabetes and type 2 diabetes | August 2021[29] | Neither[2,5] | Yes[29] | No |
| Preeclampsia | April 2017[30] | Neither[2,5] | Yes[30] | No |
| Rh(D) incompatibility | February 2004[31] | Neither[2,5] | Yes[31] | No |
| Skin cancer | July 2016[32] | Cancer[2] | No[32] | No |
| Testicular cancer | April 2011[33] | Cancer[2] | No[33] | No |
| Thyroid cancer | May 2017[34] | Cancer[2] | No[34] | No |
| Unhealthy drug use | June 2020[35] | Neither[2,5] | Yes[35] | No |
| Vision in children | September 2017[36] | Neither[2,5] | Yes[36] | No |

***Note:*** *The diseases listed in this table are those that satisfy one or both of the inclusion criteria defined in Section 2.1 of the manuscript — i.e., (1) the disease must be a cancer or an STD and (2) the USPSTF must have assigned a grade of C or higher to the screening service for the disease for at least some individuals.*

# Table S2: Lifetime number of screening occasions for each disease by subpopulation

***Female subpopulations***

| Disease | Screening procedure | FB | FP1 | FP2 | FS | FSP1 | FSP2 |
|---|---|---|---|---|---|---|---|
| Breast cancer | Mammogram | 13 | 13 | 13 | 13 | 13 | 13 |
| Cervical cancer | Pap test | 15 | 15 | 15 | 15 | 15 | 15 |
| Chlamydia | NAAT | 4 | 4 | 4 | 4 | 4 | 4 |
| Colorectal cancer | Colonoscopy | 4 | 4 | 4 | 4 | 4 | 4 |
| Gonorrhea | NAAT | 4 | 4 | 4 | 4 | 4 | 4 |
| Hepatitis B | HBsAg test | 0 | 1 | 2 | 0 | 1 | 2 |
| Hepatitis C | Anti-HCV antibody test | 1 | 2 | 3 | 1 | 2 | 3 |
| HIV | Antigen/antibody test | 1 | 2 | 3 | 1 | 2 | 3 |
| Lung cancer | Low-dose CT scan | 0 | 0 | 0 | 1 | 1 | 1 |
| Prostate cancer | PSA test | 0 | 0 | 0 | 0 | 0 | 0 |
| Syphilis | RPR test | 0 | 1 | 2 | 0 | 1 | 2 |

| | | | | |
|---|---|---|---|---|
| ***Key:*** | ***FB*** | *Baseline females* | ***FS*** | *Female smokers* |
| | ***FP1*** | *Females, one pregnancy* | ***FSP1*** | *Female smokers, one pregnancy* |
| | ***FP2*** | *Females, two pregnancies* | ***FSP2*** | *Female smokers, two pregnancies* |

### *Male subpopulations*

| Disease | Screening procedure | MB | MSM | MS | MSMS | MP | MSMP | MPS | MSMPS |
|---|---|---|---|---|---|---|---|---|---|
| Breast cancer | Mammogram | 0 | 0 | 0 | 0 | 0 | 0 | 0 | 0 |
| Cervical cancer | Pap test | 0 | 0 | 0 | 0 | 0 | 0 | 0 | 0 |
| Chlamydia | NAAT | 0 | 6 | 0 | 6 | 0 | 6 | 0 | 6 |
| Colorectal cancer | Colonoscopy | 4 | 4 | 4 | 4 | 4 | 4 | 4 | 4 |
| Gonorrhea | NAAT | 0 | 6 | 0 | 6 | 0 | 6 | 0 | 6 |
| Hepatitis B | HBsAg test | 0 | 0 | 0 | 0 | 0 | 0 | 0 | 0 |
| Hepatitis C | Anti-HCV antibody test | 1 | 1 | 1 | 1 | 1 | 1 | 1 | 1 |
| HIV | Antigen/antibody test | 1 | 6 | 1 | 6 | 1 | 6 | 1 | 6 |
| Lung cancer | Low-dose CT scan | 0 | 0 | 1 | 1 | 0 | 0 | 1 | 1 |
| Prostate cancer | PSA test | 0 | 0 | 0 | 0 | 8 | 8 | 8 | 8 |
| Syphilis | RPR test | 0 | 6 | 0 | 6 | 0 | 6 | 0 | 6 |

| | | | | |
|---|---|---|---|---|
| ***Key:*** | ***MB*** | *Baseline males* | ***MP*** | *Males, routine prostate exams* |
| | ***MSM*** | *Men who have sex with men* | ***MSMP*** | *MSM, routine prostate exams* |
| | ***MS*** | *Male smokers* | ***MPS*** | *Male smokers, routine prostate exams* |
| | ***MSMS*** | *MSM smokers* | ***MSMPS*** | *MSM smokers, routine prostate exams* |

# Table S3: Data collection procedure for each disease

| Disease | Data collection procedure |
|---|---|
| Breast cancer | 2016 USPSTF recommendation statement[1] → 2002 USPSTF evidence summary[37] → Mushlin et al 1998[38] (**Malmo**, **Swedish Two-County**) → Baines et al 1988[39] (**Canadian**), Frisell et al 1986[40] (**Stockholm**) |
| Cervical cancer | 2018 USPSTF recommendation statement[3] → 2018 USPSTF evidence review[41] (**ARTISTIC round 1**, **ARTISTIC round 2**, **FINNISH**, **NTCC phase I**, **NTCC phase II**, **POBASCAM round 1**, **POBASCAM round 2**, **SWEDESCREEN**) |
| Chlamydia | 2014 USPSTF recommendation statement[4] → 2014 USPSTF evidence review[42] (**Chernesky 2005**, **Gaydos 2013**, **Schacter 2003**, **Schoeman 2012**, **Shrier 2004**, **Taylor 2011**, **Taylor 2012**, **Van Der Pol 2012a**) |
| Colorectal cancer | 2021 USPSTF recommendation[6] → 2021 USPSTF evidence review[43] (**Zalis 2012**) |
| Gonorrhea | 2014 USPSTF recommendation statement[4] → 2014 USPSTF evidence review[42] (**Chernesky 2005**, **Gaydos 2013**, **Stewart 2012**, **Taylor 2012**, **Van Der Pol 2012a**, **Van Der Pol 2012b**) |
| Hepatitis B | 2020 USPSTF recommendation statement[7] → 2009 USPSTF reaffirmation recommendation statement[44] → 2004 USPSTF recommendation statement[45] → 2004 USPSTF evidence review[46] → 1996 USPSTF recommendation statement[47] → McCready et al 1991[48] (**McCready 1991**), Toplikar et al 1993[49] (**Toplikar 1993**) |
| Hepatitis C | 2020 USPSTF recommendation statement[9] → 2013 USPSTF recommendation statement[50] → 2004 USPSTF recommendation statement[51] → 2004 USPSTF evidence review[52] (**Huber 1996**, **Prince 1997**) → Colin et al 2001[53] (**Couroucé 1994**, **Janot 1994**, **Lavanchy 1996**, **Stuyver 1996**) |
| HIV | 2019 USPSTF recommendation statement[10] → Branson et al 2014[54] (**Bentsen 2011**, **Chavez 2011**, **Dubravac 2013**, **Masciotra 2011**, **Nasrullah 2013**, **Product insert 2010**, **Product insert 2011**) |
| Lung cancer | 2021 USPSTF recommendation statement[11] → 2021 USPSTF evidence review[55] (**Becker 2015**, **De Koning 2020**, **Infante 2015**, **Lopes Pegna 2013**, **Pinsky 2013**, **Sverzellati 2016**) |
| Prostate cancer | 2018 USPSTF recommendation statement[12] → 2018 USPSTF evidence review[56] → 2012 USPSTF recommendation statement[57] → 2011 USPSTF evidence review[58] → 2008 USPSTF recommendation statement[59] → Gann et al 1995[60] (**Gann 1995**)<br><br>2008 USPSTF evidence update[61] → 2002 USPSTF recommendation statement[62] → 2002 USPSTF evidence update[63] → Mettlin et al 1996[64] (**Mettlin 1996**), Jacobsen et al 1996[65] (**Jacobsen 1996**) |
| Syphilis | 2016 USPSTF recommendation statement (nonpregnant adults and adolescents)[13] → 2016 USPSTF evidence review (nonpregnant adults and adolescents)[66] → Ratnam 2005[67] → Larsen et al 1998[68] → Pettit et al 1983[69] (**Pettit 1983**)<br><br>2018 USPSTF recommendation statement (pregnant women)[14] → 2018 USPSTF evidence review (pregnant women)[70] → Wang et al 2016[71] (**Wang 2016**), Liu et al 2014[72] (**Liu 2014**) |

***Note:*** *Bold text denotes the study IDs from the data set.*[73]

## Table S4: Estimated lifetime false positive probability by subpopulation, cancers only and STDs only

| | *Cancers only* | *STDs only* |
|---|---|---|
| **Subpopulation** | **Estimate (SE)** | **Estimate (SE)** |
| Baseline females | 85.0% (0.9%) | 3.9% (0.2%) |
| Females, one pregnancy | 85.0% (0.9%) | 7.3% (0.4%) |
| Females, two pregnancies | 85.0% (0.9%) | 10.5% (0.5%) |
| Female smokers | 88.1% (0.7%) | 3.9% (0.2%) |
| Female smokers, one pregnancy | 88.1% (0.7%) | 7.3% (0.4%) |
| Female smokers, two pregnancies | 88.1% (0.7%) | 10.5% (0.5%) |
| Baseline males | 38.2% (3.7%) | 1.2% (0.2%) |
| Men who have sex with men (MSM) | 38.2% (3.7%) | 8.0% (0.3%) |
| Male smokers | 50.9% (2.9%) | 1.2% (0.2%) |
| MSM smokers | 50.9% (2.9%) | 8.0% (0.3%) |
| Males, routine prostate exams | 73.9% (1.7%) | 1.2% (0.2%) |
| MSM, routine prostate exams | 73.9% (1.7%) | 8.0% (0.3%) |
| Male smokers, routine prostate exams | 79.3% (1.3%) | 1.2% (0.2%) |
| MSM smokers, routine prostate exams | 79.3% (1.3%) | 8.0% (0.3%) |

# Table S5: Estimated lifetime false positive probability for each disease by subpopulation

***Female subpopulations***

| Disease | Screening procedure | FB | FP1 | FP2 | FS | FSP1 | FSP2 |
|---|---|---|---|---|---|---|---|
| Breast cancer | Mammogram | 47.7% (0.4%) | 47.7% (0.4%) | 47.7% (0.4%) | 47.7% (0.4%) | 47.7% (0.4%) | 47.7% (0.4%) |
| Cervical cancer | Pap test | 53.5% (0.4%) | 53.5% (0.4%) | 53.5% (0.4%) | 53.5% (0.4%) | 53.5% (0.4%) | 53.5% (0.4%) |
| Chlamydia | NAAT | 2.0% (0.1%) | 2.0% (0.1%) | 2.0% (0.1%) | 2.0% (0.1%) | 2.0% (0.1%) | 2.0% (0.1%) |
| Colorectal cancer | Colonoscopy | 38.2% (3.7%) | 38.2% (3.7%) | 38.2% (3.7%) | 38.2% (3.7%) | 38.2% (3.7%) | 38.2% (3.7%) |
| Gonorrhea | NAAT | 0.8% (0.1%) | 0.8% (0.1%) | 0.8% (0.1%) | 0.8% (0.1%) | 0.8% (0.1%) | 0.8% (0.1%) |
| Hepatitis B | HBsAg test | x | 2.0% (0.1%) | 4.1% (0.3%) | x | 2.0% (0.1%) | 4.1% (0.3%) |
| Hepatitis C | Anti-HCV antibody test | 1.0% (0.2%) | 1.9% (0.3%) | 2.9% (0.5%) | 1.0% (0.2%) | 1.9% (0.3%) | 2.9% (0.5%) |
| HIV | Antigen/antibody test | 0.2% (<0.1%) | 0.4% (<0.1%) | 0.6% (0.1%) | 0.2% (<0.1%) | 0.4% (<0.1%) | 0.6% (0.1%) |
| Lung cancer | Low-dose CT scan | x | x | x | 20.7% (0.1%) | 20.7% (0.1%) | 20.7% (0.1%) |
| Prostate cancer | PSA test | x | x | x | x | x | x |
| Syphilis | RPR test | x | 0.3% (<0.1%) | 0.6% (0.1%) | x | 0.3% (<0.1%) | 0.6% (0.1%) |

| | | | | |
|---|---|---|---|---|
| ***Key:*** | ***FB*** | *Baseline females* | ***FS*** | *Female smokers* |
| | ***FP1*** | *Females, one pregnancy* | ***FSP1*** | *Female smokers, one pregnancy* |
| | ***FP2*** | *Females, two pregnancies* | ***FSP2*** | *Female smokers, two pregnancies* |

### *Male subpopulations*

| Disease | Screening procedure | MB | MSM | MS | MSMS | MP | MSMP | MPS | MSMPS |
|---|---|---|---|---|---|---|---|---|---|
| Breast cancer | Mammogram | x | x | x | x | x | x | x | x |
| Cervical cancer | Pap test | x | x | x | x | x | x | x | x |
| Chlamydia | NAAT | x | 3.0% (0.2%) | x | 3.0% (0.2%) | x | 3.0% (0.2%) | x | 3.0% (0.2%) |
| Colorectal cancer | Colonoscopy | 38.2% (3.7%) | 38.2% (3.7%) | 38.2% (3.7%) | 38.2% (3.7%) | 38.2% (3.7%) | 38.2% (3.7%) | 38.2% (3.7%) | 38.2% (3.7%) |
| Gonorrhea | NAAT | x | 1.2% (0.2%) | x | 1.2% (0.2%) | x | 1.2% (0.2%) | x | 1.2% (0.2%) |
| Hepatitis B | HBsAg test | x | x | x | x | x | x | x | x |
| Hepatitis C | Anti-HCV antibody test | 1.0% (0.2%) | 1.0% (0.2%) | 1.0% (0.2%) | 1.0% (0.2%) | 1.0% (0.2%) | 1.0% (0.2%) | 1.0% (0.2%) | 1.0% (0.2%) |
| HIV | Antigen/antibody test | 0.2% (<0.1%) | 1.2% (0.1%) | 0.2% (<0.1%) | 1.2% (0.1%) | 0.2% (<0.1%) | 1.2% (0.1%) | 0.2% (<0.1%) | 1.2% (0.1%) |
| Lung cancer | Low-dose CT scan | x | x | 20.7% (0.1%) | 20.7% (0.1%) | x | x | 20.7% (0.1%) | 20.7% (0.1%) |
| Prostate cancer | PSA test | x | x | x | x | 57.9% (1.1%) | 57.9% (1.1%) | 57.9% (1.1%) | 57.9% (1.1%) |
| Syphilis | RPR test | x | 1.9% (0.2%) | x | 1.9% (0.2%) | x | 1.9% (0.2%) | x | 1.9% (0.2%) |

| Key: | | | | |
|---|---|---|---|---|
| | ***MB*** | *Baseline males* | ***MP*** | *Males, routine prostate exams* |
| | ***MSM*** | *Men who have sex with men* | ***MSMP*** | *MSM, routine prostate exams* |
| | ***MS*** | *Male smokers* | ***MPS*** | *Male smokers, routine prostate exams* |
| | ***MSMS*** | *MSM smokers* | ***MSMPS*** | *MSM smokers, routine prostate exams* |

## Section S1: Details about lifetime number of screening occasions

The number of times that individuals are recommended to get screened in a lifetime varies by subpopulation for each disease. For some diseases, it is straightforward to derive the lifetime number of screening occasions from the USPSTF guidelines. This is the case for breast cancer, as biennial mammography for women aged 50 to 74 implies 13 mammograms in a lifetime for each female subpopulation.[1] The same is true for cervical cancer — a woman who gets screened with a Pap test every three years between the ages of 21 and 65 will receive 15 Pap tests in a lifetime.[3] It is also true for colorectal cancer, as an individual who gets a colonoscopy every ten years between the ages of 45 and 75 will receive a lifetime total of four colonoscopies.[6]

For other diseases, the USPSTF guidelines lack either an age range, an interval at which screening should be repeated, or both. In these ambiguous cases, we adopt a conservative approach by imposing assumptions that are more likely to underestimate, rather than overestimate, the lifetime number of screening occasions for a particular subpopulation. This approach ensures that our estimates do not overstate the lifetime risk of a false positive. In fact, for the cases described below where we adopt this conservative approach, our estimates should be interpreted as lower bounds — i.e., the lifetime probability of a false positive for these diseases is at least as high as our estimates.

Unlike the USPSTF cancer screening guidelines, the USPSTF guidelines for the STDs do not specify an age range or an interval at which screening should be repeated. Rather, they suggest that screening should be contingent on new or persistent risk factors or that, in the cases of HIV[10] and hepatitis C,[9] repeated screening is not necessary for most individuals. We eliminate this ambiguity for several STDs by imposing the assumption that females and men who have sex with men receive one test per sexual partner, of which we assume there are four[74] for females and six[75] for MSM in a lifetime, on average. This assumption is not relevant for the non-MSM male subpopulations because these individuals are not presumed to be at increased risk for any of the STDs considered.

Another complication arising from the STD screening guidelines is that the USPSTF and CDC[76] recommend additional tests during each pregnancy for most STDs, usually at the first prenatal visit (although high-risk pregnant women may benefit from repeated screening closer to delivery). The exceptions to this are chlamydia and gonorrhea, for which the USPSTF finds no evidence of substantial net benefits from screening average-risk pregnant women[4] and the CDC only advocates additional tests for average-risk pregnant women under 25,[76] which is younger than the mean age of pregnancy in the United States.[77] As such, we assume one

additional screening occasion per pregnancy for hepatitis B, hepatitis C, HIV, and syphilis and no additional screening occasions per pregnancy for chlamydia and gonorrhea.

Finally, we employ our conservative approach when determining the number of screening occasions recommended in a lifetime for lung cancer and prostate cancer. For lung cancer, the USPSTF recommends annual screening with low-dose computed tomography for individuals between the ages of 50 and 80 who have a 20 pack-year history and who either currently smoke or have quit within the past 15 years;[11] this implies 31 screening occasions in a lifetime for eligible individuals. However, since the estimated false positive rate of each low-dose CT scan is more than 20% (see Table 1 in the manuscript), a healthy individual is almost certain to receive at least one false positive from 31 low-dose CT scans. In turn, the probability that a smoker will receive at least one false positive from any screening procedure in a lifetime also approaches 100%. Because of this, and because lung cancer screening is recognized as a service with low uptake,[11] we instead assume that male and female smokers receive only one low-dose CT scan in a lifetime. For prostate cancer, the USPSTF endorses optional screening for males between the ages of 55 and 69, but notes that there is limited evidence regarding the optimal screening interval for this service.[12] We assume that males who elect to get screened for prostate cancer do so every two years, as recommended by the American Cancer Society[78] and the American Urological Association.[79]

## Section S2: Derivation of $P_{id}$

Suppose a healthy individual in subpopulation $i$ gets screened the recommended number of times $T_{id}$ for disease $d$ in their lifetime. We aim to derive the probability $P_{id}$ that this individual will receive at least one false positive for disease $d$ in their lifetime.

For all $j \in \{1, 2, ..., T_{id}\}$, let $A_j$ denote the event where the individual receives a false positive the $j$th time they get screened for disease $d$. Note that $P_{id}$ can be thought of as the probability that at least one of $A_1, A_2, ..., A_{T_{id}}$ occurs. Therefore:

$$P_{id} = P(A_1 \cup A_2 \cup ... \cup A_{T_{id}}) = 1 - (P(A_1 \cup A_2 \cup ... \cup A_{T_{id}}))^c$$

By De Morgan's law, we have:

$$... = 1 - P(A_1^c \cap A_2^c \cap ... \cap A_{T_{id}}^c)$$

By our assumption that the results of the $T_{id}$ screening occasions are independent (see Section 2.4 of the manuscript), we have:

$$... = 1 - P(A_1^c) \cdot P(A_2^c) \cdot ... \cdot P(A_{T_{id}}^c) = 1 - (1 - P(A_1)) \cdot (1 - P(A_2)) \cdot ... \cdot (1 - P(A_{T_{id}}))$$

Recall from Section 2.3 that $p_d$ denotes the probability that a healthy individual will receive a false positive for disease $d$ from one screening occasion. It follows that for all $j \in \{1, 2, ..., T_{id}\}$, $P(A_j) = p_d$. Therefore:

$$... = 1 - (1 - p_d) \cdot (1 - p_d) \cdot ... \cdot (1 - p_d) = 1 - (1 - p_d)^{T_{id}}$$

Thus, we arrive at equation (2) from Section 2.4:

$$\boxed{P_{id} = 1 - (1 - p_d)^{T_{id}}}$$

## Section S3: Derivation of $p_i$

Recall from Section 2.4 of the manuscript that $\mathcal{D}_i$ denotes the set of diseases for which an individual in subpopulation $i$ is recommended to get screened at least once. Let $|\mathcal{D}_i|$ denote the size of the set $\mathcal{D}_i$. Suppose a healthy individual in subpopulation $i$ gets screened the recommended number of times in their lifetime for all diseases in $\mathcal{D}_i$. We seek to derive the probability $p_i$ that this individual will receive at least one false positive for at least one of the diseases in $\mathcal{D}_i$ in their lifetime.

For all $k \in \{1, 2, ..., |\mathcal{D}_i|\}$, let $B_k$ denote the event where the individual receives at least one false positive in a lifetime for the $k$th disease in $\mathcal{D}_i$. Note that $p_i$ can be thought of as the probability that at least one of $B_1, B_2, ..., B_{|\mathcal{D}_i|}$ occurs. Therefore:

$$p_i = P(B_1 \cup B_2 \cup ... \cup B_{|\mathcal{D}_i|}) = 1 - (P(B_1 \cup B_2 \cup ... \cup B_{|\mathcal{D}_i|}))^c$$

By De Morgan's law, we have:

$$... = 1 - P(B_1^c \cap B_2^c \cap ... \cap B_{|\mathcal{D}_i|}^c)$$

Recall our assumption from Section 2.4 that the event of receiving at least one false positive in a lifetime for each disease in $\mathcal{D}_i$ is independent from the same event for each of the other diseases in $\mathcal{D}_i$. Therefore:

$$... = 1 - P(B_1^c) \cdot P(B_2^c) \cdot ... \cdot P(B_{|\mathcal{D}_i|}^c) = 1 - (1 - P(B_1)) \cdot (1 - P(B_2)) \cdot ... \cdot (1 - P(B_{|\mathcal{D}_i|}))$$

Recall also that $P_{id}$ denotes the probability that a healthy individual in subpopulation $i$ will receive at least one false positive in a lifetime for some disease $d \in \mathcal{D}_i$. Let $d_1, d_2, ..., d_{|\mathcal{D}_i|}$ denote the diseases in $\mathcal{D}_i$. It follows that for all $k \in \{1, 2, ..., |\mathcal{D}_i|\}$, $P(B_k) = P_{id_k}$. Therefore:

$$... = 1 - (1 - P_{id_1}) \cdot (1 - P_{id_2}) \cdot ... \cdot (1 - P_{id_{|\mathcal{D}_i|}}) = 1 - \prod_{d \in \mathcal{D}_i} (1 - P_{id})$$

Thus, we arrive at equation (3) from Section 2.4. We can plug in $P_{id} = 1 - (1 - p_d)^{T_{id}}$ to obtain the full expression presented in Section 2.4:

$$\boxed{p_i = 1 - \prod_{d \in \mathcal{D}_i} (1 - P_{id}) = 1 - \prod_{d \in \mathcal{D}_i} (1 - p_d)^{T_{id}}}$$

## References


[1] Siu AL, U.S. Preventive Services Task Force. Screening for breast cancer: U.S. Preventive Services Task Force recommendation statement. Ann Intern Med. 2016; 164: 279-296.

[2] National Cancer Institute. Cancer Types. [cited 15 Jun 2022]. Available from: https://www.cancer.gov/types

[3] Curry SJ, Krist AH, Owens DK, Barry MJ, Caughey AB, Davidson KW, et al. Screening for cervical cancer: US Preventive Services Task Force recommendation statement. JAMA. 2018; 320: 674-686.

[4] LeFevre ML, U.S. Preventive Services Task Force. Screening for chlamydia and gonorrhea: U.S. Preventive Services Task Force recommendation statement. Ann Intern Med. 2014; 161: 902-910.

[5] Centers for Disease Control and Prevention. Diseases & Related Conditions. [cited 15 Jun 2022]. Available from: https://www.cdc.gov/std/general/default.htm

[6] Davidson KW, Barry MJ, Mangione CM, Cabana M, Caughey AB, Davis EM, et al. Screening for colorectal cancer: US Preventive Services Task Force recommendation statement. JAMA. 2021; 325: 1965-1977.

[7] Krist AH, Davidson KW, Mangione CM, Barry MJ, Cabana M, Caughey AB, et al. Screening for hepatitis B virus infection in adolescents and adults: US Preventive Services Task Force recommendation statement. JAMA. 2020; 324: 2415-2422.

[8] Owens DK, Davidson KW, Krist AH, Barry MJ, Cabana M, Caughey AB, et al. Screening for hepatitis B virus infection in pregnant women: US Preventive Services Task Force reaffirmation recommendation statement. JAMA. 2019; 322: 349-354.

[9] Owens DK, Davidson KW, Krist AH, Barry MJ, Cabana M, Caughey AB, et al. Screening for hepatitis C virus infection in adolescents and adults: US Preventive Services Task Force recommendation statement. JAMA. 2020; 323: 970-975.

[10] Owens DK, Davidson KW, Krist AH, Barry MJ, Cabana M, Caughey AB, et al. Screening for HIV infection: US Preventive Services Task Force recommendation statement. JAMA. 2019; 321: 2326-2336.

[11] Krist AH, Davidson KW, Mangione CM, Barry MJ, Cabana M, Caughey AB, et al. Screening for lung cancer: US Preventive Services Task Force recommendation statement. JAMA. 2021; 325: 962-970.

[12] Grossman DC, Curry SJ, Owens DK, Bibbins-Domingo K, Caughey AB, Davidson KW, et al. Screening for prostate cancer: US Preventive Services Task Force recommendation statement. JAMA. 2018; 319: 1901-1913.

[13] Bibbins-Domingo K, Grossman DC, Curry SJ, Davidson KW, Epling JW Jr, García FA, et al. Screening for syphilis infection in nonpregnant adults and adolescents: US Preventive Services Task Force recommendation statement. JAMA. 2016; 315: 2321-2327.

[14] Curry SJ, Krist AH, Owens DK, Barry MJ, Caughey AB, Davidson KW, et al. Screening for syphilis infection in pregnant women: US Preventive Services Task Force reaffirmation recommendation statement. JAMA. 2018; 320: 911-917.

[15] Owens DK, Davidson KW, Krist AH, Barry MJ, Cabana M, Caughey AB, et al. Screening for abdominal aortic aneurysm: US Preventive Services Task Force recommendation statement. JAMA. 2019; 322: 2211-2218.

[16] Owens DK, Davidson KW, Krist AH, Barry MJ, Cabana M, Caughey AB, et al. Screening for asymptomatic bacteriuria in adults: US Preventive Services Task Force recommendation statement. JAMA. 2019; 322: 1188-1194.

[17] Moyer VA, US Preventive Services Task Force. Screening for bladder cancer: US Preventive Services Task Force recommendation statement. Ann Intern Med. 2011;155: 246-251.

[18] Siu AL, U.S. Preventive Services Task Force. Screening for depression in children and adolescents: U.S. Preventive Services Task Force recommendation statement. Ann Intern Med. 2016; 164: 360-366.

[19] Siu AL, Bibbins-Domingo K, Grossman DC, Baumann LC, Davidson KW, Ebell M, et al. Screening for depression in adults: US Preventive Services Task Force recommendation statement. JAMA. 2016; 315: 380-387.

[20] Bibbins-Domingo K, Grossman DC, Curry SJ, Davidson KW, Epling JW Jr, García FA, et al. Serologic screening for genital herpes infection: US Preventive Services Task Force recommendation statement. JAMA. 2016; 316: 2525-2530.

[21] Davidson KW, Barry MJ, Mangione CM, Cabana M, Caughey AB, Davis EM, et al. Screening for gestational diabetes: US Preventive Services Task Force recommendation statement. JAMA. 2021; 326: 531-538.

[22] Krist AH, Davidson KW, Mangione CM, Cabana M, Caughey AB, Davis EM, et al. Screening for hypertension in adults: US Preventive Services Task Force reaffirmation recommendation statement. JAMA. 2021; 325: 1650-1656.

[23] Curry SJ, Krist AH, Owens DK, Barry MJ, Caughey AB, Davidson KW, et al. Screening for intimate partner violence, elder abuse, and abuse of vulnerable adults: US Preventive Services Task Force final recommendation statement. JAMA. 2018; 320: 1678-1687.

[24] Bibbins-Domingo K, Grossman DC, Curry SJ, Bauman L, Davidson KW, Epling JW Jr, et al. Screening for latent tuberculosis infection in adults: US Preventive Services Task Force recommendation statement. JAMA. 2016; 316: 962-969.

[25] Moyer VA, US Preventive Services Task Force. Screening for oral cancer: US Preventive Services Task Force recommendation statement. Ann Intern Med. 2014; 160: 55-60.

[26] Curry SJ, Krist AH, Owens DK, Barry MJ, Caughey AB, Davidson KW, et al. Screening for osteoporosis to prevent fractures: US Preventive Services Task Force recommendation statement. JAMA. 2018; 319: 2521-2531.

[27] Grossman DC, Curry SJ, Owens DK, Barry MJ, Davidson KW, Doubeni CA, et al. Screening for ovarian cancer: US Preventive Services Task Force recommendation statement. JAMA. 2018; 319: 588-594.

[28] Owens DK, Davidson KW, Krist AH, Barry MJ, Cabana M, Caughey AB, et al. Screening for pancreatic cancer: US Preventive Services Task Force reaffirmation recommendation statement. JAMA. 2019; 322: 438-444.

[29] Davidson KW, Barry MJ, Mangione CM, Cabana M, Caughey AB, Davis EM, et al. Screening for prediabetes and type 2 diabetes: US Preventive Services Task Force recommendation statement. JAMA. 2021; 326: 736-743.

[30] Bibbins-Domingo K, Grossman DC, Curry SJ, Barry MJ, Davidson KW, Doubeni CA, et al. Screening for preeclampsia: US Preventive Services Task Force recommendation statement. JAMA. 2017; 317: 1661-1667.

[31] US Preventive Services Task Force. Rh(D) incompatibility: Screening. 2004 [cited 15 Jun 2022]. Available from: https://www.uspreventiveservicestaskforce.org/uspstf/recommendation/rh-d-incompatibility-screening

[32] Bibbins-Domingo K, Grossman DC, Curry SJ, Davidson KW, Ebell M, Epling JW Jr, et al. Screening for skin cancer: US Preventive Services Task Force recommendation statement. JAMA. 2016; 316: 429-435.

[33] US Preventive Services Task Force. Screening for testicular cancer: US Preventive Services Task Force reaffirmation recommendation statement. Ann Intern Med. 2011; 154: 483-486.

[34] Bibbins-Domingo K, Grossman DC, Curry SJ, Barry MJ, Davidson KW, Doubeni CA, et al. Screening for thyroid cancer: US Preventive Services Task Force recommendation statement. JAMA. 2017; 317: 1882-1887.

[35] Krist AH, Davidson KW, Mangione CM, Barry MJ, Cabana M, Caughey AB, et al. Screening for unhealthy drug use: US Preventive Services Task Force recommendation statement. JAMA. 2020; 323: 2301-2309.

[36] Grossman DC, Curry SJ, Owens DK, Barry MJ, Davidson KW, Doubeni CA, et al. Vision screening in children aged 6 months to 5 years: US Preventive Services Task Force recommendation statement. JAMA. 2017; 318: 836-844.

[37] Humphrey LL, Helfand M, Chan BKS, Woolf SH. Breast cancer screening: a summary of the evidence for the U.S. Preventive Services Task Force. Ann Intern Med. 2002; 137: 347-360.

[38] Mushlin AI, Kouides RW, Shapiro DE. Estimating the accuracy of screening mammography: a meta-analysis. Am J Prev Med. 1998; 14: 143-153.

[39] Baines CJ, McFarlane DV, Miller AB. Sensitivity and specificity of first screen mammography in 15 NBSS centres. Can Assoc Radiol J. 1988; 39: 273-276.

[40] Frisell J, Glas U, Hellstrom L, Somell A. Randomized mammographic screening for breast cancer in Stockholm. Breast Cancer Res Treat. 1986; 8: 45-54.

[41] Melnikow J, Henderson JT, Burda BU, Senger CA, Durbin S, Soulsby MA. Screening for Cervical Cancer With High-Risk Human Papillomavirus Testing: A Systematic Evidence Review for the U.S. Preventive Services Task Force. Rockville, MD: Agency for Healthcare Research and Quality; 2018.

[42] Nelson HD, Zakher B, Cantor A, Deagas M, Pappas M. Screening for Gonorrhea and Chlamydia: Systematic Review to Update the U.S. Preventive Services Task Force Recommendations. Rockville, MD: Agency for Healthcare Research and Quality; 2014.

[43] Lin JS, Perdue LA, Henrikson NB, Bean SI, Blasi PR. Screening for Colorectal Cancer: An Evidence Update for the U.S. Preventive Services Task Force. Rockville, MD: Agency for Healthcare Research and Quality; 2021.

[44] US Preventive Services Task Force. Screening for hepatitis B virus infection in pregnancy: U.S. Preventive Services Task Force reaffirmation recommendation statement. Ann Intern Med. 2009; 150: 869-873.

[45] US Preventive Services Task Force. Hepatitis B virus infection: Screening. 2004 [cited 15 Jun 2022]. Available from: https://www.uspreventiveservicestaskforce.org/uspstf/recommendation/hepatitis-b-virus-infection-screening-2004

[46] US Preventive Services Task Force. Final evidence review: Hepatitis B virus infection: Screening. 2004 [cited 15 Jun 2022]. Available from: https://www.uspreventiveservicestaskforce.org/uspstf/document/final-evidence-review46/hepatitis-b-virus-infection-screening-2004

[47] US Preventive Services Task Force. Hepatitis B virus infection: Screening, 1996. 1996 [cited 15 Jun 2022]. Available from: https://www.uspreventiveservicestaskforce.org/uspstf/recommendation/hepatitis-b-virus-infection-screening-1996

[48] McCready JA, Morens D, Fields HA, Coleman PJ, Kane M, Schatz G. Evaluation of enzyme immunoassay (EIA) as a screening method for hepatitis B markers in an open population. Epidemiol Infect. 1991; 107: 673-684.

[49] Toplikar E, Carlomagno A, Rojkin LF, Gariglio R, Lorenzo LE. Development of an enzyme immunoassay for the detection of hepatitis B surface antigen employing monoclonal antibodies. J Clin Lab Anal. 1993; 7: 324-328.

[50] Moyer VA. Screening for hepatitis C virus infection in adults: U.S. Preventive Services Task Force recommendation statement. Ann Intern Med. 2013; 159: 349-357.

[51] US Preventive Services Task Force. Hepatitis C virus infection: Screening, 2004. 2004 [cited 15 Jun 2022]. Available from: https://www.uspreventiveservicestaskforce.org/uspstf/recommendation/hepatitis-c-virus-infection-screening-2004

[52] Chou R, Clark EC, Helfand M. Screening for hepatitis C virus infection: a review of the evidence for the U.S. Preventive Services Task Force. Ann Intern Med. 2004; 140: 465-479.

[53] Colin C, Lanoir D, Touzet S, Meyaud-Kraemer L, Bailly F, Trepo C, et al. Sensitivity and specificity of third-generation hepatitis C virus antibody detection assays: an analysis of the literature. J Viral Hepat. 2001; 8: 87-95.

[54] Branson BM, Owen SM, Wesolowski LG, Berry B, Werner BG, Wroblewski KE, et al. Laboratory testing for the diagnosis of HIV infection: updated recommendations. Centers for Disease Control and Prevention; 2014.

[55] Jonas DE, Reuland DS, Reddy SM, Nagle M, Clark SD, Weber RP, et al. Screening for Lung Cancer With Low-Dose Computed Tomography: An Evidence Review for the U.S. Preventive Services Task Force. Rockville, MD: Agency for Healthcare Research and Quality; 2021.

[56] Fenton JJ, Weyrich MS, Durbin S, Liu Y, Bang H, Melnikow J. Prostate-Specific Antigen-Based Screening for Prostate Cancer: A Systematic Evidence Review for the U.S. Preventive Services Task Force. Rockville, MD: Agency for Healthcare Research and Quality; 2018.

[57] Moyer VA, U.S. Preventive Services Task Force. Screening for prostate cancer: U.S. Preventive Services Task Force recommendation statement. Ann Intern Med. 2012; 157: 120-134.

[58] Lin K, Croswell JM, Koenig H, Lam C, Maltz A. Prostate-Specific Antigen-Based Screening for Prostate Cancer: An Evidence Update for the U.S. Preventive Services Task Force. Rockville, MD: Agency for Healthcare Research and Quality; 2011.

[59] U.S. Preventive Services Task Force. Screening for prostate cancer: U.S. Preventive Services Task Force recommendation statement. Ann Intern Med. 2008; 149: 185-191.

[60] Gann PH, Hennekens CH, Stampfer MJ. A prospective evaluation of plasma prostate-specific antigen for detection of prostatic cancer. JAMA. 1995; 273: 289-294.

[61] Lin K, Lipsitz R, Miller T, Janakiraman S. Benefits and Harms of Prostate-Specific Antigen Screening for Prostate Cancer: An Evidence Update for the U.S. Preventive Services Task Force. Rockville, MD: Agency for Healthcare Research and Quality; 2008.

[62] US Preventive Services Task Force. Prostate cancer: Screening, 2002. 2002 [cited 15 Jun 2022]. Available from: https://www.uspreventiveservicestaskforce.org/uspstf/recommendation/prostate-cancer-screening-2002

[63] Harris R, Lohr KN. Screening for prostate cancer: an update of the evidence for the U.S. Preventive Services Task Force. Ann Intern Med. 2002; 137: 917-929.

[64] Mettlin C, Murphy GP, Babaian RJ, Chesley A, Kane RA, Littrup PJ, et al. The results of a five-year early prostate cancer detection intervention. Cancer. 1996; 77: 150-159.

[65] Jacobsen SJ, Bergstralh EJ, Guess HA, Katusic SK, Klee GG, Oesterling JE, et al. Predictive properties of serum-prostate-specific antigen testing in a community-based setting. Arch Intern Med. 1996; 156: 2462-2468.

[66] Cantor A, Nelson HD, Daeges M, Pappas M. Screening for Syphilis in Nonpregnant Adolescents and Adults: Systematic Review to Update the 2004 U.S. Preventive Services Task Force Recommendation. Rockville, MD: Agency for Healthcare Research and Quality; 2016.

[67] Ratnam S. The laboratory diagnosis of syphilis. Can J Infect Dis Med Microbiol. 2005; 16: 45-51.

[68] Larsen SA, Pope V, Johnson RE, Kennedy EJ Jr. A Manual of Tests for Syphilis. Washington DC: American Public Health Association; 1998.

[69] Pettit DE, Larsen SA, Harbec PS, Feeley JC, Parham CE, Cruce DD, et al. Toluidine red unheated serum test, a nontreponemal test for syphilis. J Clin Microbiol. 1983; 18: 1141-1145.

[70] Lin JS, Eder M, Bean S. Screening for Syphilis Infection in Pregnant Women: A Reaffirmation Evidence Update for the U.S. Preventive Services Task Force. Rockville, MD: Agency for Healthcare Research and Quality; 2018.

[71] Wang KD, Xu DJ, Su JR. Preferable procedure for the screening of syphilis in clinical laboratories in China. Infect Dis (Lond). 2016; 48: 26-31.

[72] Liu LL, Lin LR, Tong ML, Zhang HL, Huang SJ, Chen YY, et al. Incidence and risk factors for the prozone phenomenon in serologic testing for syphilis in a large cohort. Clin Infect Dis. 2014; 59: 384-389.

[73] White T. The False Positives Calculator. 2021 [cited 15 Jun 2022]. Available from: https://falsepositives.shinyapps.io/calculator

[74] Centers for Disease Control and Prevention. Key Statistics from the National Survey of Family Growth - N Listing. [cited 15 Jun 2022]. Available from: https://www.cdc.gov/nchs/nsfg/key_statistics/n.htm

[75] Mercer CH, Prah P, Field N, Tanton C, Macdowall W, Clifton S, et al. The health and well-being of men who have sex with men (MSM) in Britain: Evidence from the third National Survey of Sexual Attitudes and Lifestyles (Natsal-3). BMC Public Health. 2016; 16: 1-16.

[76] Centers for Disease Control and Prevention. Recommended Clinician Timeline for Screening for Syphilis, HIV, HBV, HCV, Chlamydia, and Gonorrhea. [cited 15 Jun 2022]. Available from: https://www.cdc.gov/nchhstp/pregnancy/screening/clinician-timeline.html

[77] Organisation for Economic Co-operation and Development. SF2.3: Age of mothers at childbirth and age-specific fertility. 2021 [cited 15 Jun 2022]. Available from: https://www.oecd.org/els/soc/SF_2_3_Age_mothers_childbirth.pdf

[78] American Cancer Society. American Cancer Society Recommendations for Prostate Cancer Early Detection. [cited 15 Jun 2022]. Available from: https://www.cancer.org/cancer/prostate-cancer/detection-diagnosis-staging/acs-recommendations.html

[79] Carter HB, Albertsen PC, Barry MJ, Etzioni R, Freedland SJ, Greene KL, et al. Early detection of prostate cancer: AUA Guideline. J Urol. 2013; 190: 419-426.
